# Supplementary material for: Arithmetical enhancements of the Kogbetliantz method for the SVD of order two
Source: arXiv:2407.13116 ancillary file (2026-02-09)
Supplement: Supplementary file 1 [file sm.pdf]

# Arithmetical enhancements of the Kogbetliantz method for the SVD of order two: SUPPLEMENTARY MATERIAL

Vedran Novaković[†]

[*]independent researcher, Vankina ulica 15, HR-10020 Zagreb, Croatia.

Corresponding author(s). E-mail(s): venovako@venovako.eu;
[†]https://orcid.org/0000-0003-2964-9674

## 1 Direct SVD formulas for general matrices

Let $G$ be a square real matrix of order two. Find the plane rotations $U$ and $V$,

$$U = \begin{bmatrix}\cos\varphi & -\sin\varphi\\ \sin\varphi & \cos\varphi\end{bmatrix}, \qquad \cos\varphi \neq 0 \implies U = \cos\varphi\, U', \quad U' = \begin{bmatrix}1 & -\tan\varphi\\ \tan\varphi & 1\end{bmatrix},$$

$$V = \begin{bmatrix}\cos\psi & -\sin\psi\\ \sin\psi & \cos\psi\end{bmatrix}, \qquad \cos\psi \neq 0 \implies V = \cos\psi\, V', \quad V' = \begin{bmatrix}1 & -\tan\psi\\ \tan\psi & 1\end{bmatrix},$$

such that

$$U'^T G V' = \begin{bmatrix}1 & \tan\varphi\\ -\tan\varphi & 1\end{bmatrix}\begin{bmatrix}g_{11} & g_{12}\\ g_{21} & g_{22}\end{bmatrix}\begin{bmatrix}1 & -\tan\psi\\ \tan\psi & 1\end{bmatrix} = \begin{bmatrix}\sigma_1' & 0\\ 0 & \sigma_2'\end{bmatrix} = \Sigma'. \tag{1}$$

Equating the left and the right hand side in (1) gives

$$\begin{aligned}
\sigma_1' &= g_{11} + g_{21}\tan\varphi + (g_{12} + g_{22}\tan\varphi)\tan\psi, &(2)\\
0 &= g_{21} - g_{11}\tan\varphi + (g_{22} - g_{12}\tan\varphi)\tan\psi, &(3)\\
0 &= g_{12} + g_{22}\tan\varphi - (g_{11} + g_{21}\tan\varphi)\tan\psi, &(4)\\
\sigma_2' &= g_{22} - g_{12}\tan\varphi - (g_{21} - g_{11}\tan\varphi)\tan\psi. &(5)
\end{aligned}$$

From (4) it follows

$$\tan\psi = \frac{g_{12} + g_{22}\tan\varphi}{g_{11} + g_{21}\tan\varphi}, \tag{6}$$

what is substituted into (3) to get

$$(g_{11}\tan\varphi - g_{21})(g_{11} + g_{21}\tan\varphi) = (g_{22} - g_{12}\tan\varphi)(g_{12} + g_{22}\tan\varphi),$$

i.e., after grouping by $\tan\varphi$,

$$\tan\varphi(g_{11}^2 + g_{12}^2 - g_{21}^2 - g_{22}^2) = (1 - \tan^2\varphi)(g_{11}g_{21} + g_{12}g_{22}). \tag{7}$$

Dividing (7) by $(1-\tan^2\varphi)(g_{11}^2 + g_{12}^2 - g_{21}^2 - g_{22}^2)$ gives

$$\frac{\tan 2\varphi}{2} = \frac{\tan\varphi}{1-\tan^2\varphi} = \frac{g_{11}g_{21} + g_{12}g_{22}}{g_{11}^2 + g_{12}^2 - g_{21}^2 - g_{22}^2}. \tag{8}$$

Eqs. (8) and (6) are gathered into (19) from the main paper.

## 2 Single precision results

Figures 1–4 are the single precision analogues of Figures 1–4 from the main paper.

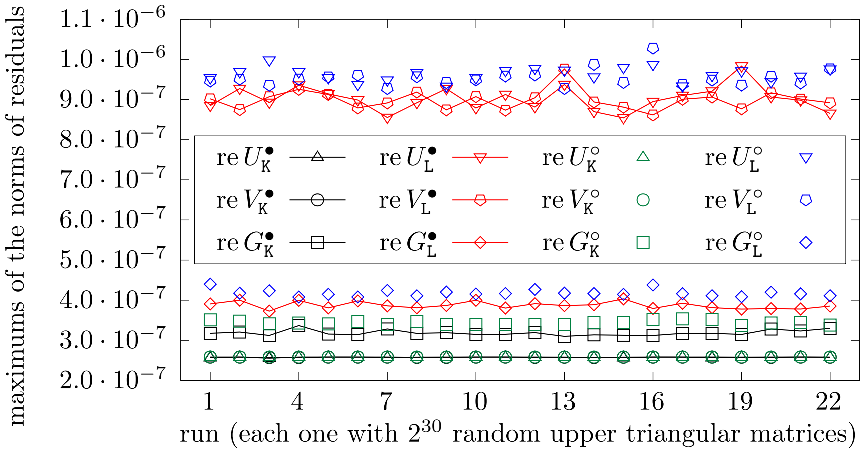


**Fig. 1** Numerical orthogonality of the singular vectors and the relative SVD residuals with `K` and `L` on random upper triangular single precision matrices.

## 3 Blocking and dynamic ordering

Blocking of the Kogbetliantz SVD for orders $n > 2$ has been discussed, e.g., in [1, 2], where [2] shows the benefits of the dynamic block-pivoting strategy. Such a strategy,

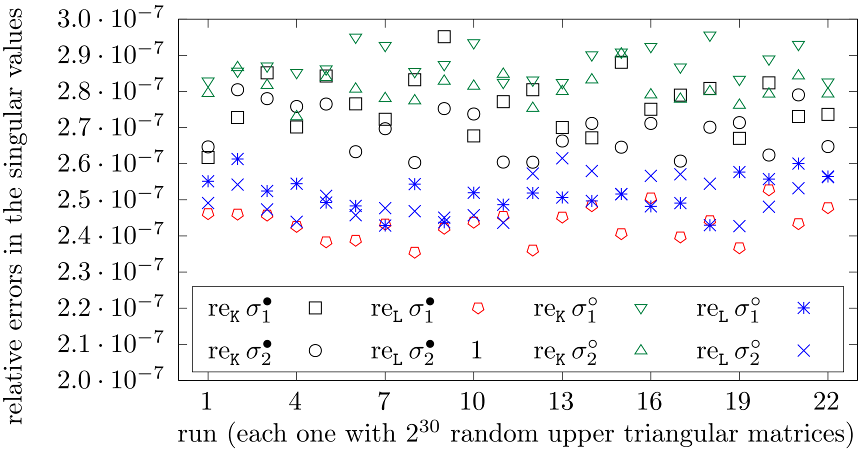


**Fig. 2** The relative errors in the singular values with `K` and `L` on random upper triangular single precision matrices, with $\max \kappa_2^{\bullet} \lessapprox 4.55 \cdot 10^{151}$ and $\max \kappa_2^{\circ} \lessapprox 9.34 \cdot 10^{10}$.

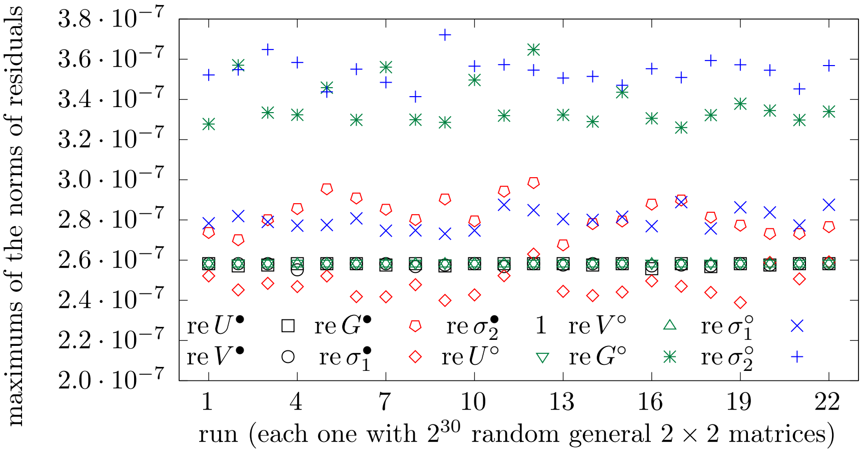


**Fig. 3** Numerical orthogonality of the singular vectors, the relative SVD residuals, and the relative errors in the singular values with `K` on random single precision matrices, with $\max \kappa_2^{\bullet} \lessapprox 2.46 \cdot 10^{81}$ and $\max \kappa_2^{\circ} \lessapprox 3.46 \cdot 10^{10}$.

in turn, requires computing or approximating the blocks' off-diagonal Frobenius norm,

$$\operatorname{off} G_{[pq]} = \sqrt{\sum_{j=l(p)}^{pb} \sum_{\substack{i=l(p)\\ i\neq j}}^{pb} |g_{ij}|^2 + \sum_{j=l(p)}^{pb} \sum_{i=l(q)}^{qb} |g_{ij}|^2 + \sum_{j=l(q)}^{qb} \sum_{i=l(p)}^{pb} |g_{ij}|^2 + \sum_{j=l(q)}^{qb} \sum_{\substack{i=l(q)\\ i\neq j}}^{qb} |g_{ij}|^2},$$
$$l(o) = (o-1)b + 1, \quad o \in \{p, q\}, \tag{9}$$

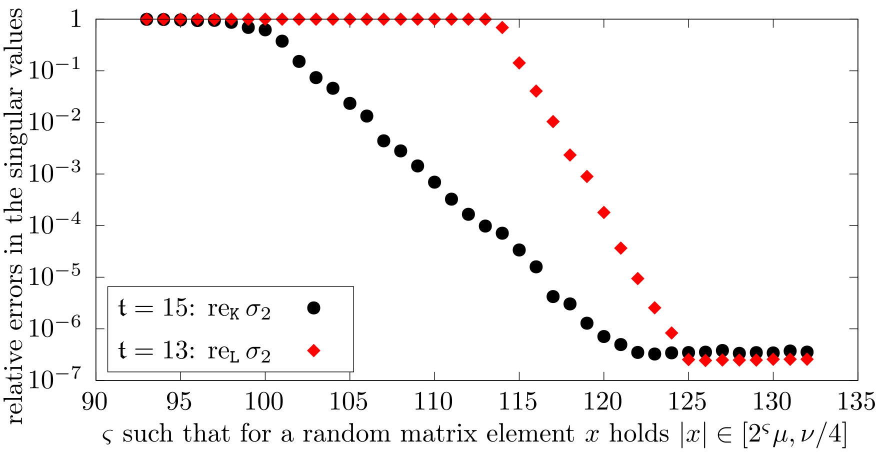


**Fig. 4** The observed decay of the relative errors in the smaller singular values by narrowing of the exponent range of the elements of single precision input matrices, where $\kappa_2^{\mathsf{K}}$ falls from $8.56 \cdot 10^{52}$ for $\varsigma = 93$ to $1.59 \cdot 10^{40}$ for $\varsigma = 132$, and $\kappa_2^{\mathsf{L}}$ from $4.28 \cdot 10^{95}$ to $1.51 \cdot 10^{72}$.

where $p$ and $q$, $1 \le p < q \le n/b$ (with $n \bmod b \equiv 0$), are block pivot indices, and $b \ge 1$ is the width of each block row and block column (so $G_{[pq]}$ blocks are of order $2b \ge 2$).

Section 3.1 offers a simple way to compute the norm (9) using hypot, Section 3.2 demonstrates some benefits of the dynamic ordering in the non-blocked (i.e., pointwise) case ($b = 1$), and Section 3.3 contains several ideas on constructing it more efficiently.

## 3.1 The Frobenius norm computation with hypot

The correctly rounded hypot provides a simple way of computing a reproducible approximation of the Frobenius norm, as Lemma 3.1 and Corollaries 3.2 and 3.3 show.

**Lemma 3.1.** Let $m \ge 1$ and let $\mathsf{x} = \begin{bmatrix} x_1 & x_2 & \cdots & x_m \end{bmatrix}^T = \mathsf{x}^{(m)}$ be a real or a complex vector. Then, its Frobenius norm $\|\mathsf{x}\|_F = \|\mathsf{x}^{(m)}\|_F$ can be computed recursively as

$$\|\mathsf{x}^{(m)}\|_F = \sqrt{\left\| \begin{bmatrix} x_1 & x_2 & \cdots & x_{m-1} \end{bmatrix}^T \right\|_F^2 + |x_m|^2} = \sqrt{\|\mathsf{x}^{(m-1)}\|_F^2 + |x_m|^2}. \tag{10}$$

*Proof.* Eq. (10) follows from the relation $\|\mathsf{x}\|_F = \sqrt{|x_1|^2 + |x_2|^2 + \cdots + |x_m|^2}$. □

**Corollary 3.2.** For a real vector $\mathsf{x}$ with $m \ge 2$ elements, $\|\mathsf{x}\|_F = \|\mathsf{x}^{(m)}\|_F$ can be approximated by the following floating-point iterations with a possible undue overflow:

$$\begin{aligned} \underline{\|\mathsf{x}^{(2)}\|_F} &= \mathrm{hypot}(\mathrm{fl}(x_1), \mathrm{fl}(x_2)); \\ \underline{\|\mathsf{x}^{(i+1)}\|_F} &= \mathrm{hypot}(\underline{\|\mathsf{x}^{(i)}\|_F}, \mathrm{fl}(x_{i+1})), \quad 2 \le i < m. \end{aligned} \tag{11}$$

*Proof.* Unwinding the recurrence (10) and the definition of hypot lead to (11). No partial norm overflows unnecessarily by itself, but a sequence of upward roundings (i.e., when rounding to nearest amounts to rounding to $+\infty$) might cause that a partial or the final norm overflows even if its exact value, correctly rounded, should not. □

**Corollary 3.3.** For a complex vector $\mathsf{x}$ with $m \ge 1$ elements, $\|\mathsf{x}\|_F = \|\mathsf{x}^{(m)}\|_F$ can be approximated by the following floating-point iterations with a possible undue overflow:

$$\underline{\|\mathsf{x}^{(1)}\|_F} = \operatorname{hypot}(\mathrm{fl}(\Re x_1), \mathrm{fl}(\Im x_1));$$
$$\underline{\|\mathsf{x}^{(i+1)}\|_F} = \operatorname{hypot}(\underline{\|\mathsf{x}^{(i)}\|_F}, \operatorname{hypot}(\mathrm{fl}(\Re x_{i+1}), \mathrm{fl}(\Im x_{i+1}))), \quad 1 \le i < m.$$

*Proof.* Similar to the proof of Corollary 3.2, using $|x_{i+1}| = \sqrt{(\Re x_{i+1})^2 + (\Im x_{i+1})^2}$. □

## 3.2 Benefits of the dynamic ordering in the pointwise case

Figure 5 compares the number of quasi-sweeps taken until convergence of the Kogbetliantz SVD with the dynamic ordering [3, 4] and the modified modulus ordering [5], showing a strong preference for the former, if it could be implemented efficiently. A quasi-sweep for the dynamic ordering is defined as a sequence of $n(n-1)/2$ sequential steps, or $n-1$ parallel steps with the maximal number of pivot pairs in each one.

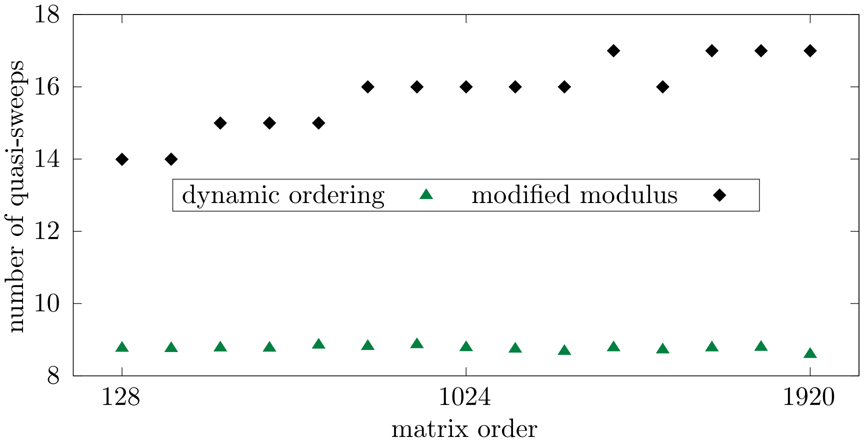


**Fig. 5** The number of quasi-sweeps taken until convergence with the dynamic ordering (approximated from the number of parallel steps) and the modified modulus ordering, over the single precision matrices that have been generated from the same singular values for each matrix order in both cases.

## 3.3 Remarks on speeding up the dynamic ordering for small $n$

The three following remarks hope to offer one possibility of speeding up the building of a parallel step under the dynamic ordering, by compactly representing the indices and the associated weights, allowing for their easy and fast comparison and sorting.

**Remark 1.** Let $x$ be a finite single precision value, and $y$ a double precision variable holding the exact value of $x$. Then at least $p_{\mathsf{D}} - p_{\mathsf{S}} = 29$ lowest bits of the significand of $y$ are zero. A quadruple precision ($p = 113$) variable $y$ can hold a double precision value $x$ while having at least 60 rightmost bits zero. Thus, a double (quadruple) precision

variable can hold an exact single (double) precision value and any payload of at most 29 (60) bits, if the payload is zeroed out before extracting the stored value of $x$.

**Remark 2.** For $(p,q)$, $1 \le p < q \le 2^d$, let $w_{pq} = \underline{\operatorname{off} G_{[pq]}}$. Then, due to Remark 1, $(w_{pq}, p, q)$ can be encoded by a single value of a higher-precision datatype that has at least $2d$ rightmost bits of the significand zero after representing $w_{pq}$ exactly. For example, the value of $p-1$ as an unsigned integer fits into the rightmost $d$ bits, and the value of $q-1$ into the next $d$ bits to the left. This defines a total order on all $(w_{pq}, p, q)$ triplets so encodable, if their encodings are compared by a usual ordering for the values of their type `x`. Since every encoding is a finite value ($w_{pq}$ is finite in higher precision), and thus not a NaN, any floating-point operator $\ge_{\mathtt{x}}$ can be taken to define

$$\operatorname{enc}(w_{pq}, p, q) \ge_{\mathtt{x}} \operatorname{enc}(w_{p'q'}, p', q') \implies (w_{pq}, p, q) \ge (w_{p'q'}, p', q'), \qquad (12)$$

where enc is the described encoding function (let the decoding function be denoted by dec). Each triplet thus requires twice the storage space of $w_{pq}$ for its encoding. Two encodings can be compared by a single floating-point operation. The enc and dec functions and the comparisons (12) are the only places where mixed-precision computation is used. This suggestion is a performance optimization, not a necessity, since the triplets can be compared semantically equivalently, but more laboriously componentwise. Note that $\operatorname{enc}(w_{pq}, p, q) \ge_{\mathtt{x}} \operatorname{enc}(w_{p'q'}, p', q')$ if and only if $w_{pq} > w_{p'q'}$, or $w_{pq} = w_{p'q'}$ and $q > q'$, or $w_{pq} = w_{p'q'}$, $q = q'$, and $p \ge p'$, with the equality of encodings being equivalent to the componentwise equality of the triplets. Up to five comparisons ($>$, $\ge$, or $=$) of the components can thus be replaced by one $\ge_{\mathtt{x}}$ comparison of the encodings, what might speed up sorting a collection of such triplets.

**Remark 3.** With the advent of hardware-supported quadruple precision (e.g., on the IBM's Power architecture), the dynamic ordering can thus rely on such encodings for matrices of orders up to $2^{30}$. This is merely a theoretical result, since in practice the dynamic ordering would be impractically slow for large matrix orders. However, a pointwise Kogbetliantz kernel with the dynamic ordering could be applied to small blocks of a large matrix to build accurate block transformations, while the outer level of blocking could use a less demanding (e.g., quasi-cyclic) strategy to select the pivot block rows and block columns to be transformed, or the dynamic ordering again [2].

# 4 A preliminary numerical comparison with `xGESVJ`

Figure 6 summarizes a preliminary numerical comparison of the Kogbetliantz SVD with `DGESVJ` (or `J` for short) on the matrices from [6], as mentioned in the main paper.

Figure 7 shows that with single precision matrices from [6] the results are more in favor of `SGESVJ`, what remains to be explained. Also, `K` is slower than `J` in single precision at the moment, so it is not recommended in this case until further polishing.

# References

[1] Bujanović, Z., Drmač, Z.: A contribution to the theory and practice of the block Kogbetliantz method for computing the SVD. BIT **52**(4), 827–849 (2012) https://doi.org/10.1007/s10543-012-0388-y

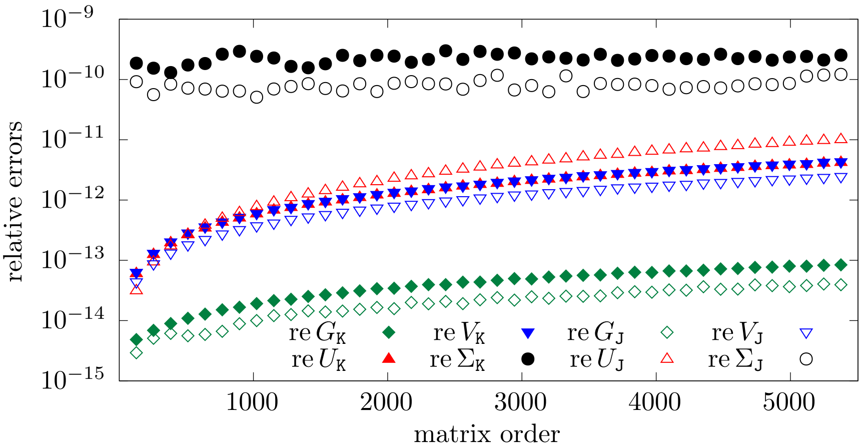


**Fig. 6** A comparison of K and J on highly conditioned matrices of order $n = 128i$, $1 \leq i \leq 42$.

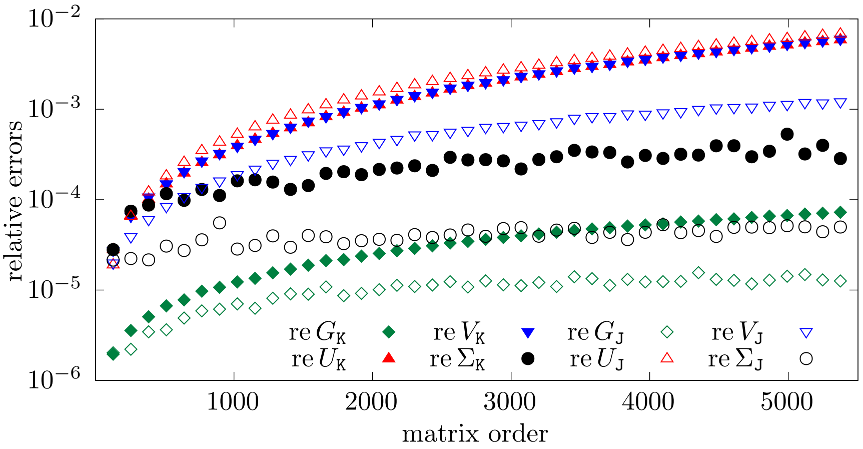


**Fig. 7** A comparison of K and J on single precision matrices of order $n = 128i$, $1 \leq i \leq 42$.


[2] Okša, G., Yamamoto, Y., Vajteršic, M.: Convergence to singular triplets in the two-sided block-Jacobi SVD algorithm with dynamic ordering. SIAM J. Matrix Anal. Appl. **43**(3), 1238–1262 (2022) https://doi.org/10.1137/21M1411895

[3] Bečka, M., Okša, G., Vajteršic, M.: Dynamic ordering for a parallel block-Jacobi SVD algorithm. Parallel Comp. **28**(2), 243–262 (2002) https://doi.org/10.1016/S0167-8191(01)00138-7

[4] Novaković, V., Singer, S.: A Kogbetliantz-type algorithm for the hyperbolic SVD. Numer. Algorithms **90**(2), 523–561 (2022) https://doi.org/10.1007/s11075-021-01197-4

[5] Novaković, V., Singer, S.: A GPU-based hyperbolic SVD algorithm. BIT **51**(4),

1009–1030 (2011) https://doi.org/10.1007/s10543-011-0333-5

[6] Novaković, V.: Vectorization of a thread-parallel Jacobi singular value decomposition method. SIAM J. Sci. Comput. **45**(3), 73–100 (2023) https://doi.org/10.1137/22M1478847
